# Supplementary material for: Reward Machines for Deep RL in Noisy and Uncertain Environments
Source: arXiv:2406.00120 source file (2025-01-15)
Supplement: Supplementary file 1 [file appendix-pastRMwork.tex]

\commentsm{This (optional) section of the appendix contains our efforts to expand (very briefly) upon the related work on RMs that is mentioned in the introduction, as promised in our author response. \begin{itemize}
    \item We can decide whether to include it once we see how far we get. 
    \item We should also consider its placement within the appendix and 
    \item we should make reference to it in the Introduction, if we decide to keep it
\end{itemize}    
    }

\noindent {\bf Text from Intro:}\\
For these reasons, formal languages, and in particular, Reward Machines, have been adopted across a diversity of domains, ranging from motion planning \citep{kress2009temporal, fainekos2009temporal, sun2024neurosymbolic} and robotic manipulation \citep{camacho2021reward,he2015towards, kunze2011logic} to, more recently, general deep Reinforcement Learning (RL) problems %over large inputs 
\citep[e.g.,][]{aksaray2016q,li2017reinforcement,li2018policy, littman2017environment,icarte2018using,tor-etal-neurips19, hasanbeig2018logically,deeplcrl,alur2019,DBLP:conf/ijcai/0005T19,kuo2020encoding,HasanbeigKA20Deep,xu2020joint,xu2020active,furelos2020inductionAAAI,rens2020learning,DBLP:conf/kr/GiacomoFIPR20,jiang2020temporal, neary2020reward, shah2020planning, velasquez2021learning,defazio2021learning,zheng2021lifelong,camacho2021reward,corazza2022reinforcement,liu2022skill, furelos2023hierarchies, shah2024deep, zhang2023exploiting, vaezipoor2021ltl2action, DBLP:journals/ai/IcarteKVCWM23}. 
~~\\\noindent {\bf End Text from Intro}

\noindent {\bf Verbatim related work text from JAIR paper}\\

~~\\\noindent {\bf End Text from JAIR}

\noindent {\bf Verbatim related work text from AIJ paper - perhaps not relevant}\\

~~\\\noindent {\bf End Text from AIJ}
